# Supplementary material for: Propensity of water self-ions at air(oil)-water interfaces revealed by deep potential molecular dynamics with enhanced sampling
Source: arXiv:2404.07027 ancillary file (2024-11-12)
Supplement: Supplementary file 1 [file Supporting_information.pdf]

---

# –SUPPORTING INFORMATION–

## PROPENSITY OF WATER SELF-IONS AT AIR(OIL)-WATER INTERFACES REVEALED BY DEEP POTENTIAL MOLECULAR DYNAMICS WITH ENHANCED SAMPLING

---

Pengchao Zhang<sup>1</sup>, Axel Tosello Gardini<sup>2,3</sup>, and Xuefei Xu<sup>1,\*</sup>.

<sup>1</sup>Center for Combustion Energy, Department of Energy and Power Engineering, and Key Laboratory for Thermal Science and Power Engineering of Ministry of Education, Tsinghua University, Beijing 100084, China

<sup>2</sup>Atomistic Simulations, Italian Institute of Technology, Genova 16152, Italy

<sup>3</sup>Department of Materials Science, Università di Milano-Bicocca, 20126 Milano, Italy

\*Corresponding author e-mail: xuxuefei@tsinghua.edu.cn

## 1 Computational methods

### 1.1 Potential model generation

#### 1.1.1 Constructing training datasets

The key to effective model training lies in constructing appropriate datasets. In this work, we aim to train two distinct models: a DP model for molecular dynamics simulations investigating double-layer distribution of self-ions in interfaces, and a DeePKS model with accuracy comparable to the M06-2X functional, which will be used for labeling the DP training datasets. To ensure diverse and uncorrelated data, we generate multiple independent MD simulations with enhanced sampling on some configuration systems (Table S1), including reactive processes.

The training sets for the two models differ significantly in size due to variations in their descriptors. Both models, however, adhere to the criteria of physical symmetry and locality. The DP model incorporates angular and radial atomic environment descriptors, while the DeePKS model includes gauge invariance symmetry and density matrices projected on atomic orbitals.<sup>1-3</sup> Consequently, the DeePKS model requires only a few hundred configurations for training, whereas the DP model necessitates tens of thousands to accurately capture reactive processes. The training datasets for the DeePKS and DP models consist of 600 and 69,787 configurations, respectively.

#### 1.1.2 Density functional theory (DFT) calculation

The preparation of training and test datasets for DeePKS involves using the CP2K package<sup>4</sup> to calculate M06-2X<sup>5</sup> energies and forces. These calculations utilize Goedecker-Teter-Hutter pseudopotentials<sup>6,7</sup> and a QZV3P basis set.<sup>8</sup> The multi-grid level employs a plane-wave cutoff of 1000 Ry for the total density and 70 Ry for the Kohn-Sham orbitals, as confirmed by a previous convergent test.<sup>9</sup> To speed up the convergence of self-consistent field (SCF) iterations, the auxiliary density matrix method is employed.<sup>10</sup>

#### 1.1.3 DeePKS model training

We aim to perform highly accurate simulations of energy and forces using the M06-2X functional.<sup>5</sup> However, the computational cost of single-point calculations at the M06-2X level is prohibitively high for our current system. To

address this, we employ DeePKS, a neural network framework that trains a correction term to bridge the gap between the M06-2X target energy ( $E_{\text{M06-2X}}$ ) and the more affordable PBE baseline energy ( $E_{\text{PBE}}$ ).<sup>11</sup>

The DeePKS model is generated iteratively using the DeePKS-kit.<sup>2,12,13</sup> We alternate between training the correction network from the PBE baseline to the M06-2X target and solving the resulting DeePKS model using ABACUS.<sup>3,14,15</sup> ABACUS employs optimized norm-conserving Vanderbilt pseudopotentials<sup>16</sup> and a numerical atomic orbital basis.<sup>17</sup> The calculations utilize a kinetic energy cutoff of 100 Ry and a density error SCF convergence threshold of  $1 \times 10^{-7}$  Ry.

The DeePKS model employs descriptors derived from projected density matrices, which are obtained using a predefined set of projectors with a maximum angular momentum of 2. The number of Bessel functions is determined based on radial and wavefunction cutoffs of 5 Bohr and 100 Ry, respectively. The model architecture consists of three hidden layers with 32 neurons each, and the "gelu" activation function is applied between the hidden layers. The training process involves 10,000 iterations with a learning rate ranging from  $10^{-4}$  to  $10^{-7}$ . During training processes, energy and atomic forces are estimated using a weighted mean squared loss function, i.e.,  $\mathcal{L}^{\text{DeePKS}}$

$$\mathcal{L}^{\text{DeePKS}} = |E^{\text{M06-2X}} - E^{\text{DeePKS}}(\varphi_i|w)|^2 + p |\mathbf{F}^{\text{M06-2X}} - \mathbf{F}^{\text{DeePKS}}(\varphi_i|w)|^2. \quad (\text{S1})$$

The Hamiltonian, denoted as  $\hat{H}^{\text{DeePKS}}$ , determines the energy and force in the DeePKS model.

$$\hat{H}^{\text{DeePKS}} = \hat{H}^{\text{PBE}} + \hat{H}^{\delta}. \quad (\text{S2})$$

$\hat{H}^{\text{DeePKS}}$  consists of a baseline term,  $\hat{H}^{\text{PBE}}$ , and a correction term,  $\hat{H}^{\delta}$ . The eigenstate of  $\hat{H}^{\text{DeePKS}}$ , represented by  $\varphi_i$ , partially depends on  $\hat{H}^{\delta}$ .  $\hat{H}^{\delta}$  is determined using projected density matrices, localized orbitals, and the DeePKS descriptor. The iterative process of combining  $\hat{H}^{\text{DeePKS}}$  with  $\hat{H}^{\delta}$  identifies different ground states and achieves convergence through model training and SCF solution.<sup>2,3</sup> Additionally,  $w$  represents the parameter of the neural network, and  $p$  serves as a pre-factor to compensate for errors.

Once the DeePKS model is trained, the iterative process is no longer required. Total energies and forces can be obtained through single point calculations using the PBE functional corrected for the  $E_{\delta}$  term. The PBE-based DeePKS model shows good agreement with independent testing data obtained from M06-2X/QZV3P calculations, with low root mean square errors (RMSEs) of 0.49 meV/atom in energy and 46 meV/Å in force (Fig. S2). Additionally, the PBE-based DeePKS model offers significant computational efficiency, saving nearly nine times the time compared to the standard M06-2X functional (Table S3).

#### 1.1.4 DP model training

The Deep Potential Smooth Edition descriptor<sup>1,18</sup> is utilized in this study. The embedding net is configured with layer sizes of [25, 50, 100] and employs a "tanh" activation function between hidden layers. A submatrix size of 16 is incorporated. The neighbor atom cutoff radius is set at 6.0 Å, with smoothing starting at 0.5 Å. The maximum number of neighboring atoms for H, C, and O atoms is specified as [88, 46, 45] respectively. The embedding net is followed by the fitting net, comprising layers sized at [240, 240, 240], where the "tanh" activation function is applied between hidden layers. The fitting net incorporates the ResNet architecture.<sup>19</sup> The training process consists of 10 million steps with a learning rate ranging from  $10^{-3}$  to  $10^{-8}$ . The loss function, denoted as  $\mathcal{L}^{\text{DP}}$ , combines energy and atomic forces using a weighted mean square approach

$$\mathcal{L}^{\text{DP}} = \frac{p_e}{N} |E^{\text{DeePKS}} - E^{\text{DP}}(w)|^2 + \frac{p_f}{3N} \sum_{i\alpha} |F_{i\alpha}^{\text{DeePKS}} - F_{i\alpha}^{\text{DP}}(w)|^2, \quad (\text{S3})$$

where  $N$  denotes the number of atoms,  $p_e$  and  $p_f$  are pre-factors of the energy  $E$  and force  $F$ , respectively, and  $w$  represents the parameter of the neural network.  $F_{i\alpha}$  represents the force felt by atom  $i$  in the direction of  $\alpha$ th.

The DP model is trained using the DeePMD-kit,<sup>20,21</sup> utilizing a training dataset of M06-2X quality. A total of 69,787 configurations are used for accurate results. The trained DP model is then evaluated by testing its predictions on a separate dataset, which undergoes standard M06-2X energy and force calculations. The DP model achieves energy RMSE of 0.85 meV/atom and atomic force RMSE of 58 meV/Å (Fig. S3), demonstrating a level of precision comparable to M06-2X. Furthermore, the DP model exhibits a computational speed advantage of five orders of magnitude over M06-2X-based simulations (Table S3).

## 1.2 Molecular dynamics simulations

### 1.2.1 MD simulation for the training dataset generation

The configurations (systems B-H in Table S1) used for training the DeePKS and DP models are obtained through MD simulations using CP2K,<sup>4</sup> with the exception of some pure water configurations (system A in Table S1) taken from previous work.<sup>22</sup> To speed up the sampling process, the semi-empirical method GFN1-xTB<sup>23</sup> is employed to derive the potential energy surface. The MD simulations are carried out in a constant volume constant temperature (NVT) ensemble with a time step of 1.0 fs, maintained using a velocity rescaling thermostat<sup>24</sup> at 300 K with a damping time of 0.2 ps.

### 1.2.2 DPMD simulation for studying the autoionization and the double-layer distribution

To investigate the double-layer of self-ions at water interfaces, DPMD simulations are conducted using the LAMMPS software.<sup>25</sup> Prior to simulating the interface systems, the accuracy of water autoionization in a bulk system (Table S2) is assessed through 10 ns NVT simulations with a 1.0 fs integration time step. Temperature control at 300 K is achieved using a velocity rescaling thermostat with a damping time of 0.04 ps. For the air-water and oil-water interface systems (Table S2), 30 ns simulations are performed to obtain converged results, and other simulation settings are consistent with those used for the water bulk system.

## 1.3 Enhanced sampling settings

### 1.3.1 Bias potential of enhanced sampling

In both MD simulations for constructing the datasets and the DPMD simulation, the OPES method<sup>26–28</sup> with collective variables (CVs) is employed. The CVs, denoted as  $\mathbf{s}(\mathbf{R})$ , effectively capture slow modes and infrequent occurrences by relating them to atomic coordinates  $\mathbf{R}$ . The external bias potential  $V(\mathbf{s})$  is incorporated into the system's potential energy  $U(\mathbf{R})$  during MD simulations using the PLUMED plugin.<sup>29</sup> In OPES,  $V(\mathbf{s})$  at the  $n$ th step is characterized by

$$V_n(\mathbf{s}) = (1 - \frac{1}{\gamma}) \frac{1}{\beta} \log(\frac{P_n(\mathbf{s})}{Z_n} + \epsilon), \quad (\text{S4})$$

where the expression involves the bias factor  $\gamma = \beta \Delta E_{\text{bias}}$ , inverse Boltzmann factor  $\beta = 1/k_B T$ , the unbiased marginal distribution probability  $P(\mathbf{s})$ , and a normalization factor  $Z$ . The regularization term  $\epsilon = e^{-\gamma/(1-1/\gamma)}$  ensures a positive argument for the logarithm and imposes a bias constraint that confines sampling to the specified region of interest. The adaptive kernel width is used to update the bias every 500 steps, and a value of  $\Delta E_{\text{bias}}$  of 75 kJ/mol is chosen to approximate the free energy barrier of water autoionization.

The OPES-explore variant is employed for collecting dataset configurations, as it facilitates phase space exploration in systems containing water (systems B-F in Table S1), while OPES with expanded ensembles target distribution is used to explore the phase space of pure oil systems G and H (Table S1). During the final DPMD simulation, the original OPES method generates well-converged free energy estimates (the systems as shown in Table S2). The difference in estimating probability distributions between OPES and OPES-explore arises due to their distinct approaches, although they share the concept of defining the bias potential. OPES calculates an unbiased probability  $P(\mathbf{s})$  on-the-fly using weighted kernel density estimation (KDE), while OPES-explore calculates a well-tempered probability  $p^{\text{WT}}(\mathbf{s}) \propto [P(\mathbf{s})]^{\frac{1}{\gamma}}$  based on an averaged KDE.<sup>26,27</sup>

### 1.3.2 Definition of collective variables

Protons are able to diffuse through water utilizing the Grotthuss mechanism,<sup>22,30,31</sup> in which a charge defect migrates through the hydrogen network rather than a specific proton. Therefore, any CV related to proton diffusion must be able to identify charge defects without reference to particular atomic coordinates. In this particular case, there are various possible charge defects, namely the two water self-ions  $\text{H}_3\text{O}^+$  and  $\text{OH}^-$ . To automatically identify these charge defects, we implement the methodology proposed in References<sup>9,32,33</sup> which involves tessellation of the space by Voronoi polyhedra centered on the O atoms and subsequent summation of the contained charge in each polyhedron. If the charge within a polyhedron differs from zero, we attribute the charge deficiency to the O atom located at the center of the polyhedron.

To calculate the number of hydrogen (H) atoms  $n_i$  centered on oxygen (O) atom  $i$ , utilize the specified equation

$$n_i = \sum_{j=1}^{\text{Num}_H} \frac{e^{-\lambda|\mathbf{R}_i - \mathbf{R}_j|}}{\sum_{m=1}^{\text{Num}_O} e^{-\lambda|\mathbf{R}_m - \mathbf{R}_j|}}, \quad (\text{S5})$$

where  $m$  represents the index of all Voronoi centers, and the sum includes all H atoms with index  $j$ . The parameter  $\lambda$  governs the smoothness of the function.

The charge defect of the Voronoi center,  $\delta_i$ , is calculated by subtracting the reference number,  $n_i^0$  (protons for the atom at the polyhedron center), from the H number,  $n_i$

$$\delta_i = n_i - n_i^0, \quad (\text{S6})$$

where we assume  $n_i^0 = 2$  for the oxygen (O) atom in water.

During OPES simulations to study water autoionization processes, the CV  $s_a$  with a value of  $\lambda = 5$  is utilized to obtain a smoother definition of the self-ion number, given that water self-ions ( $\text{H}_3\text{O}^+$  and  $\text{OH}^-$ ) may be present.

$$s_a = \sum_{i=1}^{\text{Num}_O} \delta_i^2, \quad (\text{S7})$$

where the process encourages autoionization in which the value of  $s_a$  ranges from 0 to  $<2$ .

The mean absolute error (MAE) between  $s_a^{\lambda=5}$  and  $s_a^{\lambda=100}$  is calculated. Although  $s_a^{\lambda=5}$  deviates slightly from 2 due to the smoothness of the function for well sampling,  $s_a^{\lambda=100}$  is much closer to 2 at autoionization state. However,  $s_a^{\lambda=100}$  is too narrow for effective sampling and reweighting. The MAE value of approximately 0.7 indicates that when  $s_a^{\lambda=5} \approx 1.3$  and  $s_a^{\lambda=100} \approx 2.0$ , they represent a pair of  $\text{H}_3\text{O}^+$  and  $\text{OH}^-$  coexisting in water.

The CV  $s_a$  is supplemented by adding a CV  $s_t$  with a value of  $\lambda = 8$  that indicates the self-ion distance between  $\text{H}_3\text{O}^+$  and  $\text{OH}^-$

$$s_t = - \sum_{i=1}^{\text{Num}_O} \sum_{j>i}^{\text{Num}_O} r_{i,j} \delta_i \delta_j, \quad (\text{S8})$$

while  $s_t$  can differentiate between the state of pure water ( $s_t \approx 0 \text{ \AA}$ ) and the state of autoionization ( $s_t > 0 \text{ \AA}$ ), its resolution around the initial transfer of proton is inadequate due to its concentration around zero. Therefore, we employ the piecewise logarithmic function

$$s'_t = \begin{cases} \log(s_t + \epsilon), & 0 \leq s_t < 1, \\ s_t - 1 + \log(1 + \epsilon), & s_t \geq 1, \end{cases} \quad (\text{S9})$$

where  $\epsilon = 0.03$  represents the regularization term. The self-ion distance variant  $s'_t$  can differentiate between the pure water state ( $s'_t \approx -3 \text{ \AA}$ ), the transition state ( $s'_t \approx 0 \text{ \AA}$ ), and the autoionization state ( $s'_t > 1 \text{ \AA}$ ).

Based on the definition of self-ion number  $s_a$ , we designed the z-axis coordinate (the interface normal vector is parallel to the z-axis direction) of  $\text{H}_3\text{O}^+$  and  $\text{OH}^-$  to explore their preferences along the interface after water autoionization.

For the negative ion ( $\text{OH}^-$ ), we represent the CV of the z-axis coordinate as  $s_{zn}$

$$s_{zn} = \sum_{i=1}^{\text{Num}_O} \delta z_i \delta_i^2 \quad (\text{for } \delta_i < 0). \quad (\text{S10})$$

For the positive ion ( $\text{H}_3\text{O}^+$ ), the z-axis coordinate CV represented by the  $s_{zp}$

$$s_{zp} = \sum_{i=1}^{\text{Num}_O} \delta z_i \delta_i^2 \quad (\text{for } \delta_i > 0), \quad (\text{S11})$$

where  $\delta z_i = |z_i - z_{\text{mid}}|$  indicates that we calculate the absolute value with respect to the central layer ( $z_{\text{mid}} = 53 \text{ \AA}$  is the middle value of the box along the z-axis) in our interface systems, which combines the top and bottom interfaces to determine the CV values.

When reweighting the unbiased possibility, we focus solely on the formation of one pair of self-ions through pure water ( $0 \leq s_a \leq 2$ ). We do not consider cases where autoionization results in the formation of more than one pair of self-ions ( $s_a > 2$ ) when calculating the free energy along the CVs  $s_{zn}$  and  $s_{zp}$ .

The uncertainty is calculated for  $s_{zn}^{\lambda=5}$  and  $s_{zn}^{\lambda=100}$ , as well as for  $s_{zp}^{\lambda=5}$  and  $s_{zp}^{\lambda=100}$ , in both the oil-water and air-water systems. In the oil-water system, the MAE value is found to be  $\sim 10$  Å. In the air-water system, the MAE value is  $\sim 9.0$  Å. This implies that the curves depicted in manuscript Fig. 2 exhibit a horizontal displacement along the x-axis within the specified range due to the smoothness of the CVs for well sampling.

Furthermore, it is worth noting that in long timescale simulations, there exists a probability for a few  $H_2O$  molecules to transition into the gas phase or return back to the water surface. Consequently, this phenomenon can lead to an underestimation of the water density, thereby introducing some errors in the determination of the middle layer and interface region. However, it is important to emphasize that these deviations do not significantly impact the overall validity and robustness of our main conclusions.

### 1.3.3 Free energy calculation

Upon completion of the DPMD simulation, the free energy surface (FES) along the CV can be calculated as follows

$$F(s) = -\frac{1}{\beta} \log P(s). \quad (S12)$$

In the regime of quasi-static bias,  $P(s)$  can be reweighted as an average over the biased ensemble.<sup>26</sup>

$$P(s) = \frac{\langle \delta[s - s(\mathbf{R})] e^{\beta V(s)} \rangle_V}{\langle e^{\beta V(s)} \rangle_V}. \quad (S13)$$

## 2 Other computational details

The simulation results are presented using VMD<sup>34</sup> and Matplotlib<sup>35</sup> packages. To investigate the minimum free energy pathways derived from the two-dimensional free energy surface, we employed the MEPSA (Minimum Energy Path Surface Analysis) package.<sup>36</sup> The diffusion coefficient of water is determined from the mean square displacement (MSD) using Einstein's relation, which was previously described.<sup>22</sup> Our M06-2X-based DPMD simulations reveal a diffusion coefficient of  $2.26 \times 10^{-9} \text{ m}^2\text{s}^{-1}$  at 300 K for water molecules, consistent with experimental results ( $\sim 2.3 \times 10^{-9} \text{ m}^2\text{s}^{-1}$ ). Additionally, the diffusion coefficients for  $H_3O^+$  and  $OH^-$  at 300 K are  $8.23 \times 10^{-9}$  and  $4.63 \times 10^{-9} \text{ m}^2\text{s}^{-1}$ , respectively, which agree well with experimental measurements ( $\sim 9 \times 10^{-9} \text{ m}^2\text{s}^{-1}$  for  $H_3O^+$  and  $\sim 5 \times 10^{-9} \text{ m}^2\text{s}^{-1}$  for  $OH^-$  at  $\sim 300$  K).<sup>37-39</sup> The simulation workflow depicted in Fig. S1 consists of six steps detailed in our earlier research.<sup>9</sup>

Table S1: **Details of the simulation systems for building training and testing datasets.** Using OPES-explore, the oil-water systems B, C, D, E, and F contain water autoionization processes to include features of  $\text{H}_3\text{O}^+$  and  $\text{OH}^-$  ions. The phase space of pure oil systems G and H is explored by OPES with expanded ensembles target distribution. The only exceptions are some pure water configurations (system A) are added from our previous work.<sup>22</sup>

| System | Box size ( $\text{\AA}^3$ )               | No. of $\text{H}_2\text{O}$ | No. of $\text{C}_{10}\text{H}_{22}$ |
|--------|-------------------------------------------|-----------------------------|-------------------------------------|
| A      | $\sim 12.2 \times 12.2 \times 12.2$ (NPT) | 64                          | 0                                   |
| B      | $12.0 \times 12.0 \times 12.0$ (NVT)      | 58                          | 0                                   |
| C      | $12.0 \times 12.0 \times 36.0$ (NVT)      | 54                          | 0                                   |
| D      | $12.5 \times 12.5 \times 12.5$ (NVT)      | 44                          | 2                                   |
| E      | $12.5 \times 12.5 \times 12.5$ (NVT)      | 22                          | 4                                   |
| F      | $12.5 \times 12.5 \times 20.0$ (NVT)      | 52                          | 5                                   |
| G      | $12.5 \times 12.5 \times 12.5$ (NVT)      | 0                           | 6                                   |
| H      | $12.5 \times 12.5 \times 12.5$ (NVT)      | 0                           | 7                                   |

Table S2: **Details of the simulation systems for performing final molecular dynamics and analysis.**

| System              | Box size ( $\text{\AA}^3$ )     | No. of $\text{H}_2\text{O}$ | No. of $\text{C}_{10}\text{H}_{22}$ |
|---------------------|---------------------------------|-----------------------------|-------------------------------------|
| Water bulk          | $12.0 \times 12.0 \times 12.0$  | 58                          | 0                                   |
| Air-water interface | $12.1 \times 12.1 \times 106.0$ | 256                         | 0                                   |
| Oil-water interface | $12.1 \times 12.1 \times 106.0$ | 256                         | 24                                  |

Table S3: **The runtime of calculations.** DFT labeling and DeePKS labeling are executed on a CPU processor with parallelization. The runtime is designated for the completion of the self-consistent field iteration. The runtime of DPMD simulation with OPES on GPU is provided.

| Step                                | System              | Machine      | Time            |
|-------------------------------------|---------------------|--------------|-----------------|
| DFT labeling for the DeePKS dataset | B                   | 24-core CPU  | 35 min/frame    |
| DeePKS labeling for the DP dataset  | B                   | 24-core CPU  | 4 min/frame     |
| DPMD simulation with OPES           | Water bulk          | 1 Tesla A100 | 127 timesteps/s |
| DPMD simulation with OPES           | Air-water interface | 1 Tesla A100 | 80 timesteps/s  |
| DPMD simulation with OPES           | Oil-water interface | 1 Tesla A100 | 65 timesteps/s  |

Table S4: **The component of the datasets.** The two models, DeePKS and DP, employ training and testing datasets that consist of a number of configurations. M06-2X/QZV3P is used to perform the DeePKS training datasets and all test datasets, while the DP training datasets are carried out using the DeePKS models. For systems C and F, the M06-2X/QZV3P method is directly used to label the DP training dataset, hence corresponding DeePKS model and test dataset are unavailable.

| System | DeePKS Train | DP Train | Test |
|--------|--------------|----------|------|
| A, B   | 150          | 23371    | 680  |
| C      | N/A          | 5997     | N/A  |
| D      | 150          | 8106     | 500  |
| E      | 150          | 8872     | 500  |
| F      | N/A          | 13682    | N/A  |
| G, H   | 150          | 9759     | 800  |
| Total  | 600          | 69787    | 2480 |

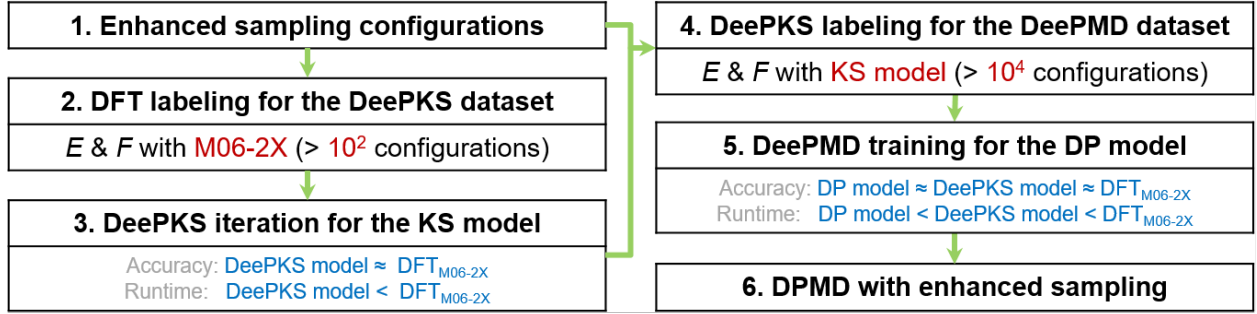

Figure S1: **Simulation workflow in detail.** The workflow involves a series of steps for efficient and accurate exploration of the double-layer distribution of water self-ions in interfaces after autoionization. The process includes enhanced sampling techniques, DFT labeling, iteration with the DeePKS model, labeling with DeePKS predictions, training the DP model, and DPMD simulations using the OPES method. This comprehensive approach allows for a thorough investigation of the double-layer distribution with improved computational efficiency and accuracy.

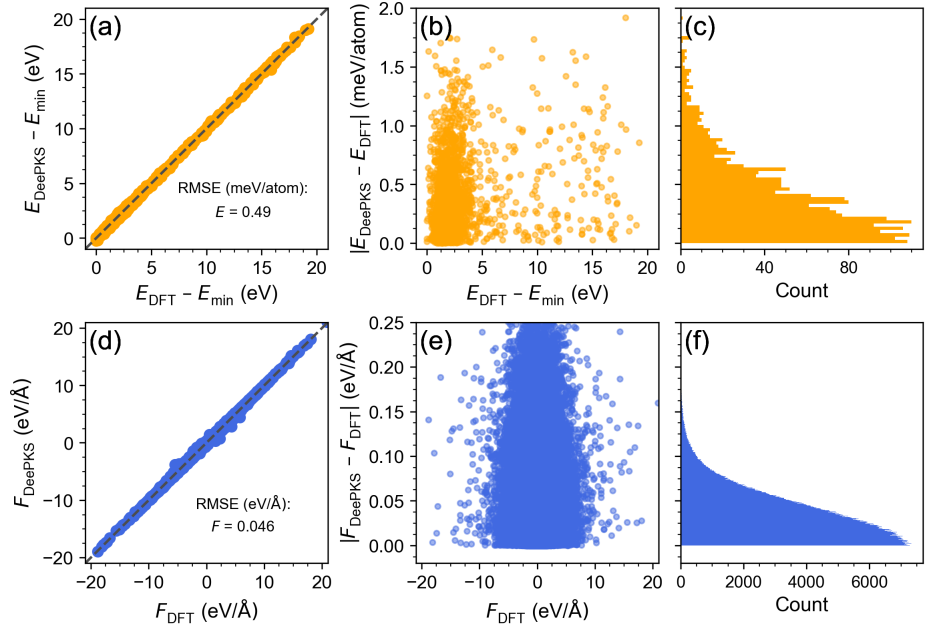

Figure S2: **Error distribution of the DeePKS model on the testing dataset.** (a) The distribution of  $E_{\text{DeePKS}} - E_{\min}$  with respect to  $E_{\text{DFT}} - E_{\min}$ . (b) Left: the distribution of  $|E_{\text{DeePKS}} - E_{\text{DFT}}|$  with respect to  $E_{\text{DFT}} - E_{\min}$ . (c) Right: the histogram of  $|E_{\text{DeePKS}} - E_{\text{DFT}}|$ . (d) The distribution of  $F_{\text{DeePKS}}$  with respect to  $F_{\text{DFT}}$ . (e) Left: the distribution of  $|F_{\text{DeePKS}} - F_{\text{DFT}}|$  with respect to  $F_{\text{DFT}}$ . (f) Right: the histogram of  $|F_{\text{DeePKS}} - F_{\text{DFT}}|$ . Here,  $E_{\text{DFT}}$  and  $F_{\text{DFT}}$  are the energy and force calculated by the M06-2X functional;  $E_{\text{DeePKS}}$  and  $F_{\text{DeePKS}}$  are the energy and force performed by the present DeePKS model; and  $E_{\min}$  is the minimum absolute energy in the testing dataset.

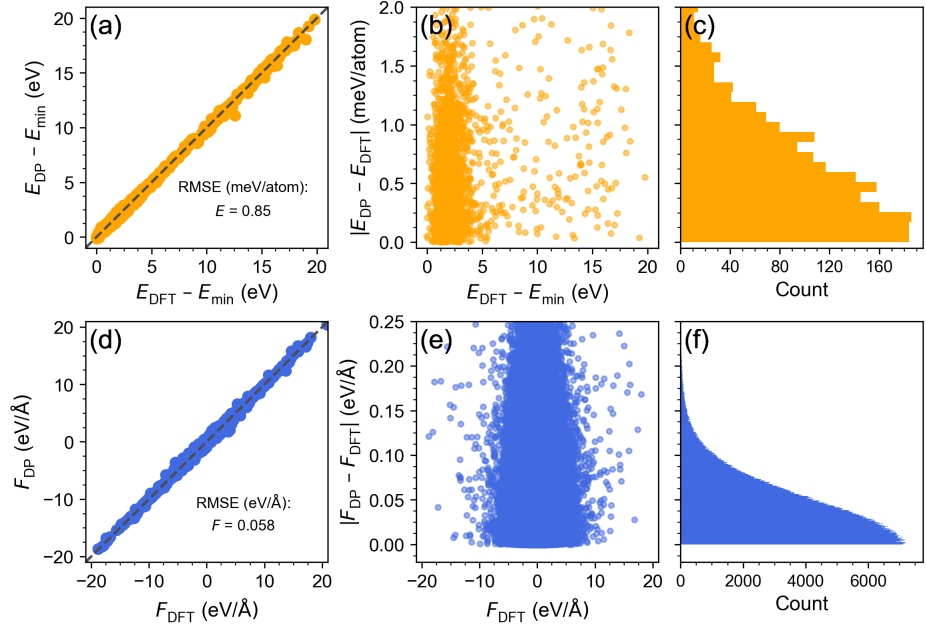

Figure S3: **Error distribution of the DP model on the testing dataset.** (a) The distribution of  $E_{\text{DP}} - E_{\text{min}}$  with respect to  $E_{\text{DFT}} - E_{\text{min}}$ . (b) Left: the distribution of  $|E_{\text{DP}} - E_{\text{DFT}}|$  with respect to  $E_{\text{DFT}} - E_{\text{min}}$ . (c) Right: the histogram of  $|E_{\text{DP}} - E_{\text{DFT}}|$ . (d) The distribution of  $F_{\text{DP}}$  with respect to  $F_{\text{DFT}}$ . (e) Left: the distribution of  $|F_{\text{DP}} - F_{\text{DFT}}|$  with respect to  $F_{\text{DFT}}$ . (f) Right: the histogram of  $|F_{\text{DP}} - F_{\text{DFT}}|$ . Here,  $E_{\text{DFT}}$  and  $F_{\text{DFT}}$  are the energy and force calculated by the M06-2X functional;  $E_{\text{DP}}$  and  $F_{\text{DP}}$  are the energy and force performed by the present DP model; and  $E_{\text{min}}$  is the minimum absolute energy in the testing dataset.

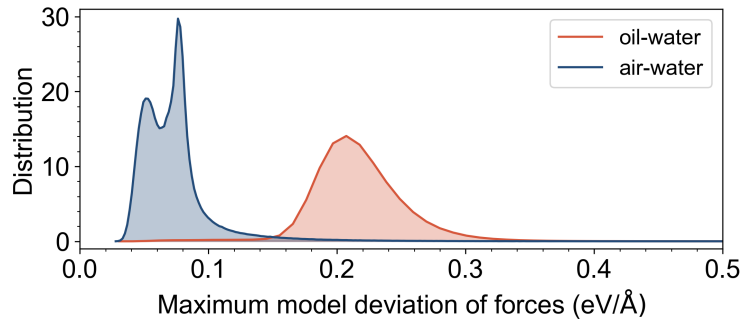

Figure S4: **Uncertainty of atomic force predictions from DPMD simulations.** The distribution of the maximum model deviation of the forces for the configurations generated by the DP models in representative MD trajectories, calculated from 4 DP models trained on different permutations of the training data set and different random seeds. This can be considered as a proxy for the uncertainty of the neural network predictions, and the deviation values less than 0.3 eV/Å indicate that our models are robust with adequate training datasets.

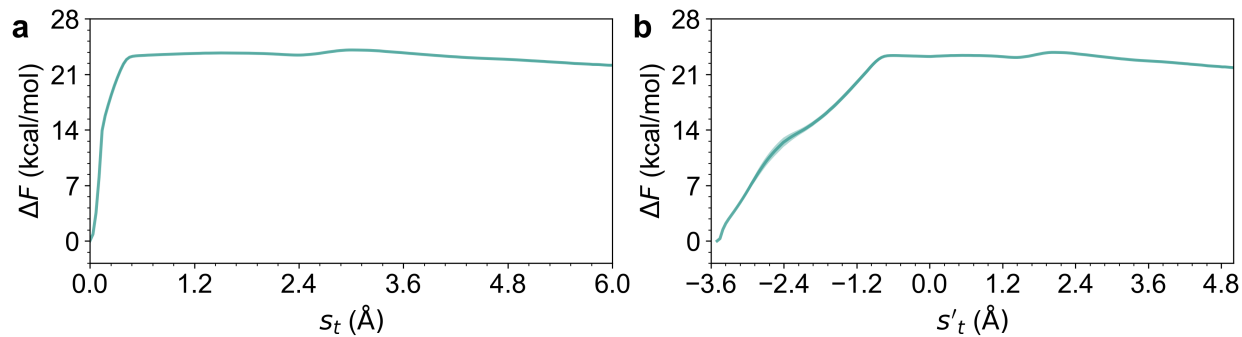

Figure S5: **Water autoionization in water bulk system.** One-dimensional projections of the FES along the CVs (a)  $s_t$  and (b)  $s'_t$ . The CVs  $s'_t$  and  $s_t$  are not sufficient to illustrate the metastable state when ions separate from each other, so we primarily focus on the FES along the self-ion number  $s_a$  as shown in the manuscript.

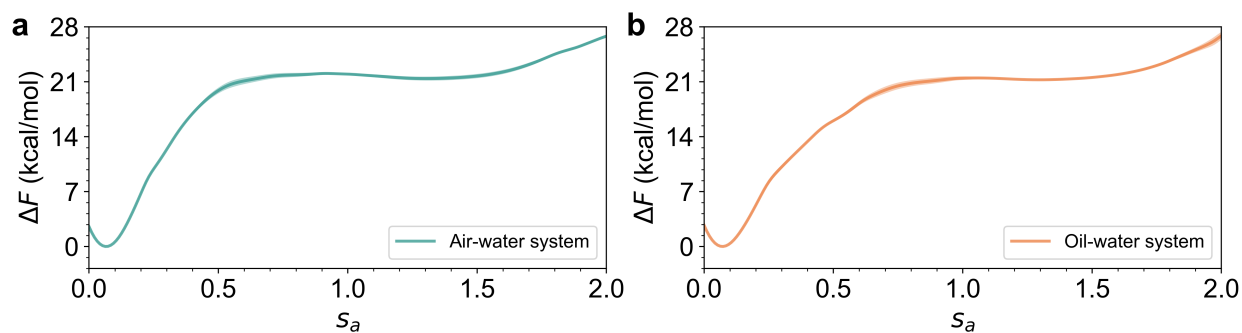

Figure S6: **Water autoionization in interface systems.** One-dimensional FES as a function of the self-ion number  $s_a$  in (a) air-water system and (b) oil-water system. Identifying transition states becomes more ambiguous in these systems due to the presence of more water molecules. The results of the reaction energy for water autoionization in 256  $H_2O$  ( $\Delta F^\circ = 21.4, 21.2$  kcal/mol in air-water, oil-water system, respectively) are consistent with those in the bulk with 58  $H_2O$  ( $\Delta F^\circ = 20.8$  kcal/mol), which means that the size effects are not significant in our cases.

## References

- [1] Zhang, L.; Han, J.; Wang, H.; Car, R.; Weinan, E. Deep potential molecular dynamics: a scalable model with the accuracy of quantum mechanics. *Physical review letters* **2018**, *120*, 143001.
- [2] Chen, Y.; Zhang, L.; Wang, H.; E, W. DeePKS: A comprehensive data-driven approach toward chemically accurate density functional theory. *Journal of Chemical Theory and Computation* **2020**, *17*, 170–181.
- [3] Li, W.; Ou, Q.; Chen, Y.; Cao, Y.; Liu, R.; Zhang, C.; Zheng, D.; Cai, C.; Wu, X.; Wang, H.; others DeePKS+ABACUS as a Bridge between Expensive Quantum Mechanical Models and Machine Learning Potentials. *The Journal of Physical Chemistry A* **2022**, *126*, 9154–9164.
- [4] Kühne, T. D.; Iannuzzi, M.; Del Ben, M.; Rybkin, V. V.; Seewald, P.; Stein, F.; Laino, T.; Khaliullin, R. Z.; Schütt, O.; Schiffmann, F.; others CP2K: An electronic structure and molecular dynamics software package-Quickstep: Efficient and accurate electronic structure calculations. *The Journal of Chemical Physics* **2020**, *152*, 194103.
- [5] Zhao, Y.; Truhlar, D. G. The M06 suite of density functionals for main group thermochemistry, thermochemical kinetics, noncovalent interactions, excited states, and transition elements: two new functionals and systematic testing of four M06-class functionals and 12 other functionals. *Theoretical chemistry accounts* **2008**, *120*, 215–241.
- [6] Goedecker, S.; Teter, M.; Hutter, J. Separable dual-space Gaussian pseudopotentials. *Physical Review B* **1996**, *54*, 1703.
- [7] Hartwigsen, C.; Goedecker, S.; Hutter, J. Relativistic separable dual-space Gaussian pseudopotentials from H to Rn. *Physical Review B* **1998**, *58*, 3641.
- [8] VandeVondele, J.; Krack, M.; Mohamed, F.; Parrinello, M.; Chassaing, T.; Hutter, J. Quickstep: Fast and accurate density functional calculations using a mixed Gaussian and plane waves approach. *Computer Physics Communications* **2005**, *167*, 103–128.
- [9] Zhang, P.; Gardini, A. T.; Xu, X.; Parrinello, M. Intramolecular and water mediated tautomerism of solvated glycine. *Journal of Chemical Information and Modeling* **2024**.
- [10] Guidon, M.; Hutter, J.; VandeVondele, J. Auxiliary density matrix methods for Hartree-Fock exchange calculations. *Journal of chemical theory and computation* **2010**, *6*, 2348–2364.
- [11] Perdew, J. P.; Burke, K.; Ernzerhof, M. Generalized gradient approximation made simple. *Physical review letters* **1996**, *77*, 3865.
- [12] Chen, Y.; Zhang, L.; Wang, H.; E, W. Ground state energy functional with Hartree-Fock efficiency and chemical accuracy. *The Journal of Physical Chemistry A* **2020**, *124*, 7155–7165.
- [13] Chen, Y.; Zhang, L.; Wang, H.; Weinan, E. DeePKS-kit: A package for developing machine learning-based chemically accurate energy and density functional models. *Computer Physics Communications* **2023**, *282*, 108520.
- [14] Chen, M.; Guo, G.; He, L. Systematically improvable optimized atomic basis sets for *ab initio* calculations. *Journal of Physics: Condensed Matter* **2010**, *22*, 445501.
- [15] Li, P.; Liu, X.; Chen, M.; Lin, P.; Ren, X.; Lin, L.; Yang, C.; He, L. Large-scale *ab initio* simulations based on systematically improvable atomic basis. *Computational Materials Science* **2016**, *112*, 503–517.
- [16] Schlipf, M.; Gygi, F. Optimization algorithm for the generation of ONCV pseudopotentials. *Computer Physics Communications* **2015**, *196*, 36–44.
- [17] Lin, P.; Ren, X.; He, L. Strategy for constructing compact numerical atomic orbital basis sets by incorporating the gradients of reference wavefunctions. *Physical Review B* **2021**, *103*, 235131.
- [18] Zhang, L.; Han, J.; Wang, H.; Saidi, W.; Car, R.; others End-to-end symmetry preserving inter-atomic potential energy model for finite and extended systems. *Advances in neural information processing systems* **2018**, *31*.
- [19] He, K.; Zhang, X.; Ren, S.; Sun, J. Deep residual learning for image recognition. Proceedings of the IEEE conference on computer vision and pattern recognition. 2016; pp 770–778.
- [20] Wang, H.; Zhang, L.; Han, J.; E, W. DeePMD-kit: A deep learning package for many-body potential energy representation and molecular dynamics. *Computer Physics Communications* **2018**, *228*, 178–184.
- [21] Zeng, J.; Zhang, D.; Lu, D.; Mo, P.; Li, Z.; Chen, Y.; Rynik, M.; Huang, L.; Li, Z.; Shi, S.; others DeePMD-kit v2: A software package for deep potential models. *The Journal of Chemical Physics* **2023**, *159*.
- [22] Zhang, P.; Feng, M.; Xu, X. Double-layer distribution of hydronium and hydroxide ions in the air-water interface. *ACS Physical Chemistry Au* **2024**.
- [23] Grimme, S.; Bannwarth, C.; Shushkov, P. A robust and accurate tight-binding quantum chemical method for structures, vibrational frequencies, and noncovalent interactions of large molecular systems parametrized for all spd-block elements (Z=1–86). *Journal of chemical theory and computation* **2017**, *13*, 1989–2009.
- [24] Bussi, G.; Donadio, D.; Parrinello, M. Canonical sampling through velocity rescaling. *The Journal of chemical physics* **2007**, *126*, 014101.
- [25] Plimpton, S. Fast parallel algorithms for short-range molecular dynamics. *Journal of computational physics* **1995**, *117*, 1–19.
- [26] Invernizzi, M.; Parrinello, M. Rethinking metadynamics: From bias potentials to probability distributions. *The journal of physical chemistry letters* **2020**, *11*, 2731–2736.
- [27] Invernizzi, M.; Parrinello, M. Exploration vs convergence speed in adaptive-bias enhanced sampling. *Journal of Chemical Theory and Computation* **2022**, *18*, 3988–3996.
- [28] Invernizzi, M.; Piaggi, P. M.; Parrinello, M. Unified approach to enhanced sampling. *Physical Review X* **2020**, *10*, 041034.
- [29] Tribello, G. A.; Bonomi, M.; Branduardi, D.; Camilloni, C.; Bussi, G. PLUMED 2: New feathers for an old bird. *Computer physics communications* **2014**, *185*, 604–613.
- [30] de Grotthuss, C. J. T. Mémoire sur la Décomposition de l'Eau et des Corps qu'elle Tient en Dissolution à l'Aide de l'Électricité Galvanique. *Ann. Chim.* **1806**, *54–74*.
- [31] Marx, D. Proton transfer 200 years after von Grotthuss: Insights from *ab initio* simulations. *ChemPhysChem* **2006**, *7*, 1848–1870.
- [32] Grifoni, E.; Piccini, G.; Parrinello, M. Microscopic description of acid-base equilibrium. *Proceedings of the National Academy of Sciences* **2019**, *116*, 4054–4057.
- [33] Grifoni, E.; Piccini, G.; Parrinello, M. Tautomeric equilibrium in condensed phases. *Journal of Chemical Theory and Computation* **2020**, *16*, 6027–6031.
- [34] Humphrey, W.; Dalke, A.; Schulten, K. VMD: visual molecular dynamics. *Journal of molecular graphics* **1996**, *14*, 33–38.
- [35] Hunter, J. D. Matplotlib: A 2D graphics environment. *Computing in science & engineering* **2007**, *9*, 90–95.
- [36] Marcos-Alcalde, I.; Setoain, J.; Mendieta-Moreno, J. I.; Mendieta, J.; Gomez-Puertas, P. MEPSA: minimum energy pathway analysis for energy landscapes. *Bioinformatics* **2015**, *31*, 3853–3855.
- [37] Halle, B.; Karlström, G. Prototropic charge migration in water. part 2.—Interpretation of nuclear magnetic resonance and conductivity data in terms of model mechanisms. *Journal of the Chemical Society, Faraday Transactions 2: Molecular and Chemical Physics* **1983**, *79*, 1047–1073.
- [38] Sluyters, J.; Sluyters-Rehbach, M. The mechanism of the hydrogen ion conduction in liquid light and heavy water derived from the temperature dependence of their limiting conductivities. *The Journal of Physical Chemistry B* **2010**, *114*, 15582–15589.
- [39] Chen, M.; Zheng, L.; Santra, B.; Ko, H.-Y.; DiStasio Jr, R. A.; Klein, M. L.; Car, R.; Wu, X. Hydroxide diffuses slower than hydronium in water because its solvated structure inhibits correlated proton transfer. *Nature chemistry* **2018**, *10*, 413–419.
